# Supplementary material for: Is Scaling Learned Optimizers Worth It? Evaluating The Value of VeLO's 4000 TPU Months
Source: arXiv:2310.18191 source file (2024-03-07)
Supplement: Supplementary file 1 [file appendix.tex]

\section{Appendix}

Optionally include extra information (complete proofs, additional experiments and plots) in the appendix.
This section will often be part of the supplemental material.
